# Supplementary material for: TEaR: Improving LLM-based Machine Translation with Systematic Self-Refinement
Source: arXiv:2402.16379 source file (2024-06-21)
Supplement: Supplementary file 1 [file appendix_module.tex]

\begin{table*}
\centering
% \vskip 0.15in
\resizebox{\textwidth}{!}{%
\begin{tabular}{cccccccccccccccccc} 
\toprule
\multicolumn{2}{c}{\textbf{Translate }} &  & \multicolumn{2}{c}{\textbf{Estimate }} &  & \multicolumn{2}{c}{\textbf{Refine }}   &  & \multirow{2}{*}{\textbf{\# of tested}} & \multirow{2}{*}{} & \multirow{2}{*}{\textbf{BLEU}} &  & \multirow{2}{*}{\textbf{COMET}} &  & \multirow{2}{*}{\textbf{COMETKiwi}} &  & \multirow{2}{*}{\textbf{BLEURT}}  \\ 
\cmidrule{1-2}\cmidrule{4-5}\cmidrule{7-8}
\textbf{0-shot} & \textbf{5-shot}       &  & \textbf{0-shot} & \textbf{3-shot}      &  & \textbf{wo 5-shot} & \textbf{w 5-shot} &  &                                        &                   &                                &  &                                 &  &                                     &  &                                   \\ 
\midrule
\checkmark             &                       &  & -               & -                    &  & -                  & -                 &  & \multirow{10}{*}{200}                  &                   & 25.45                          &  & 80.01                           &  & 78.87                               &  & 66.56                             \\
\checkmark             &                       &  & \checkmark             &                      &  & \checkmark                &                   &  &                                        &                   & 24.95                          &  & 80.05                           &  & 78.95                               &  & 66.64                             \\
\checkmark             &                       &  & \checkmark             &                      &  &                    & \checkmark               &  &                                        &                   & 25.15                          &  & 80.22                           &  & 79.18                               &  & 66.91                             \\
\checkmark             &                       &  &                 & \checkmark                  &  & \checkmark                &                   &  &                                        &                   & 25.56                          &  & 80.52                           &  & 79.75                               &  & 67.01                             \\
\checkmark             &                       &  &                 & \checkmark                  &  &                    & \checkmark               &  &                                        &                   & 25.79                          &  & 80.68                           &  & 79.77                               &  & 67.09                             \\
                & \checkmark                   &  & -               & -                    &  & -                  & -                 &  &                                        &                   & 26.30                          &  & 80.31                           &  & 79.28                               &  & 67.07                             \\
                & \checkmark                   &  & \checkmark             &                      &  & \checkmark                &                   &  &                                        &                   & 26.12                          &  & 80.44                           &  & 79.71                               &  & 67.24                             \\
                & \checkmark                   &  & \checkmark             &                      &  &                    & \checkmark               &  &                                        &                   & 26.23                          &  & 80.54                           &  & 79.94                               &  & 67.33                             \\
                & \checkmark                   &  &                 & \checkmark                  &  & \checkmark                &                   &  &                                        &                   & 26.01                          &  & 80.52                           &  & 79.79                               &  & 67.66                             \\
                & \checkmark                   &  &                 & \checkmark                  &  &                    & \checkmark               &  &                                        &                   & \textbf{26.41}                 &  & \textbf{80.70}                  &  & \textbf{\textbf{80.07}}             &  & \textbf{\textbf{67.84}}           \\
\bottomrule
\end{tabular}
}
% \vskip -0.1in
\caption{The results of testing translation ability of various LLMs under 5-shot setting in our sampled WMT23 datasets.}
\label{tab:app_module}
\end{table*}
